# Supplementary material for: High-dimensional neural network potentials for solvation: The case of protonated water clusters in helium
Source: arXiv:2103.13123 ancillary file (2021-03-24)
Supplement: Supplementary file 1 [file si.pdf]

# Supplemental Material

## High-dimensional neural network potentials for solvation: The case of protonated water clusters in helium

Christoph Schran,[1] Felix Uhl,[1] Jörg Behler,[2,1] and Dominik Marx[1]

[1]*Lehrstuhl für Theoretische Chemie, Ruhr-Universität Bochum, 44801 Bochum, Germany*

[2]*Universität Göttingen, Institut für Physikalische Chemie, Theoretische Chemie, Tammannstr. 6, 37077 Göttingen, Germany*

(Dated: September 28, 2017)

# I. COMPUTATIONAL METHODS AND DETAILS

## A. Validation of the Reference Method

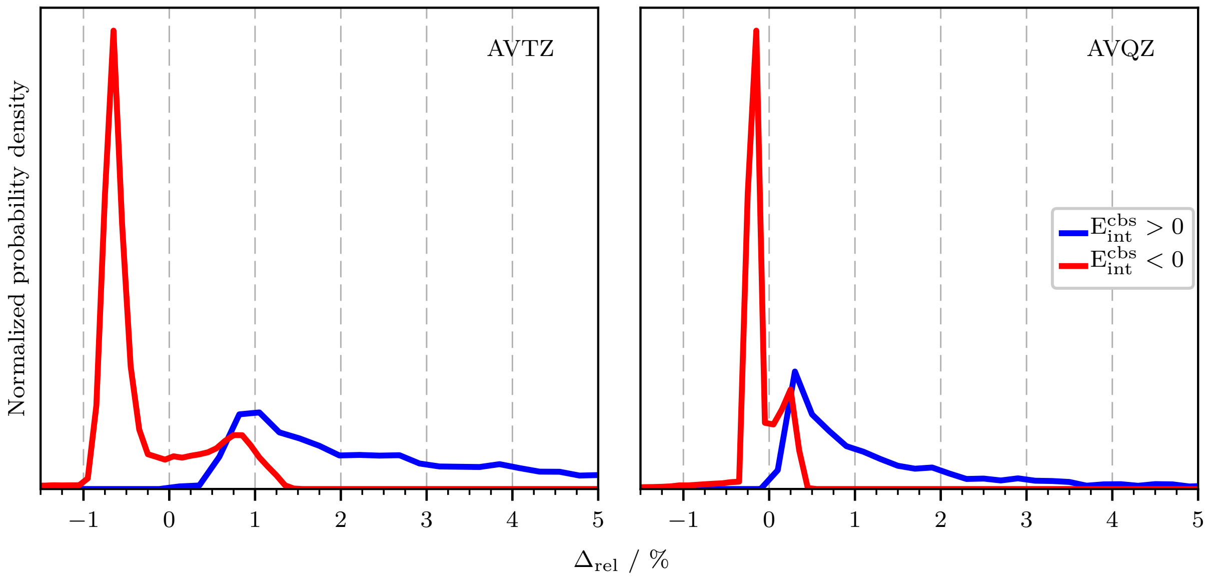


Figure S1. Distribution of the relative error $\Delta_{rel}$ in the interaction energies for 250 000 He-$H_3O^+$ configurations using the AVTZcp (left) and AVQZcp (right) basis set, see text, compared to the complete basis set (cbs) limit $E_{int}^{cbs}$ obtained with the $X^{-3}$ extrapolation scheme [1] where the red distribution accounts for attractive and the blue distribution for repulsive interaction energies $E_{int}^{cbs}$.

The CCSD(T) method features relatively slow basis set convergence. We therefore explicitly tested the quality of the reference calculations for the He-$H_3O^+$ adduct. For this purpose, we evaluated the He-solute pair CCSD(T) interaction potential of two selected frozen $H_3O^+$ configurations centered in a cubic grid with 50 helium grid points in each dimension and a grid spacing of 0.25 Å employing the aug-cc-pVTZ and aug-cc-pVQZ basis set [2, 3] together with a counterpoise correction[4] to correct for the basis set superposition error, abbreviated as AVTZcp and AVQZcp. Two $H_3O^+$ structures extracted from the reference ensemble (see main text for details), a flat one close to the transition state of the pseudorotation, and a structure close to the minimum energy structure have been selected. The complete basis set (CBS) limit was subsequently estimated using the $X^{-3}$ extrapolation scheme [1] applied directly on the interaction energies as suggested in Ref. 5. Note that extrapolation of the individual components of the interaction energy did result in negligible differences. The rel-

ative error in the interaction energy to the CBS is calculated for both basis sets according to

$$\Delta_{\text{rel}} = \frac{E_{\text{int}} - E_{\text{int}}^{\text{CBS}}}{E_{\text{int}}^{\text{CBS}}} \cdot 100 \ . \tag{S1}$$

In Fig. S1 the distribution of the relative error of the resulting 250 000 He-$H_3O^+$ adducts is shown for the AVTZcp (left) and AVQZcp (right) basis. As expected, the smaller AVTZcp basis features overall slightly larger relative errors than AVQZcp. Configurations close to the $H_3O^+$ molecule with repulsive interaction energies feature larger relative errors compared to the remaining configurations and we thus dissected the distributions accordingly. For attractive interaction energies the relative error of the AVTZcp basis is below $\pm 1$ %, while repulsive interaction energies feature much larger errors up to 5 %. Note that unlike for the individual energy components, the interaction energy can be increased as well as decreased when approaching the CBS and the relative error can thus be positive or negative. Therefore, the distributions feature two peaks for attractive interaction energies. For the larger AVQZcp basis the relative error is reduced below $\pm 0.5$ % for attractive and 3 % for repulsive interaction energies.

To estimate the influence of the basis set error when using AVTZcp, we conducted helium PIMC simulations at 1.67 K with 98 helium atoms around the clamped $H_3O^+$ configurations and evaluated the interaction potential using the nearest neighbor approach (see main text) on the grid. For all six grids, 20 Monte Carlo walkers generated 100 000 structures with 10 000 Monte Carlo steps in between and the radial distribution function (RDF) of helium were calculated. The oxygen-helium and hydrogen-helium RDFs evaluated on the grid, where the energy was obtained with the AVTZcp basis and in the CBS limit for both $H_3O^+$ structures, are compared in Fig. S2. In all four shown cases, the RDFs obtained with the AVTZcp grid are almost identical to the functions obtained on the CBS grid. This proves that the error when using the AVTZcp basis does not change the solvation structure around $H_3O^+$ on the accuracy scale that is relevant in the present case.

We conclude from this analysis that using the AVTZcp basis results in negligible basis set errors of around $\pm 0.5$ % for attractive interaction energies that do not influence the helium solvation structure around the solute molecule.

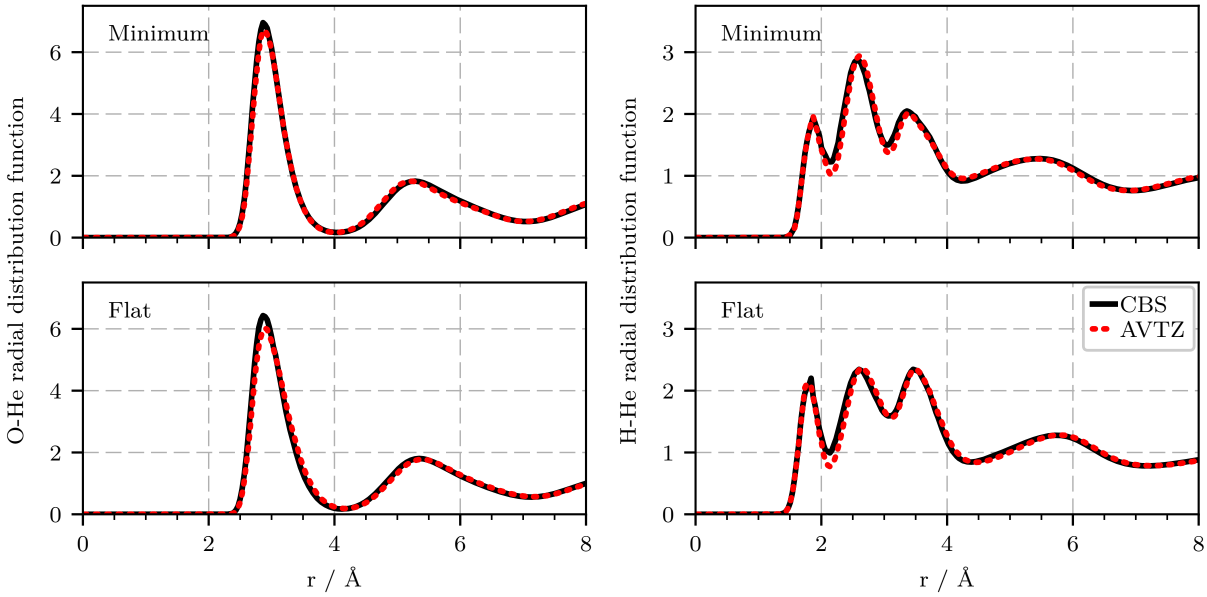


Figure S2. Radial distribution functions of two $H_3O^+$ structures ('Minimum': Top row, 'Flat': Bottom row) in bulk helium at 1.67 K obtained from PIMC simulations of helium around fixed solute structures where the interaction potential was evaluated on a grid using the AVTZcp interaction energies (red, dotted) as well as those from the CBS extrapolation (black).

## B. Radial Interaction Potential Scan

To restrict the reference calculations to the relevant parts of configuration space, we performed two radial scans of the interaction potential of the He-$H_3O^+$ complex that are depicted in Fig. S3. Helium configurations close to the solute molecule are very high in energy due to Pauli repulsion, while configurations far away from the solute molecule feature interaction energies close to zero. We therefore determined a lower cutoff radius around each atom type as well as an upper cutoff radius, where interaction energies can be assumed to be very small, for the generation of He-solute pair configurations. This consideration results in the following radial ranges

$$r_{\text{X-He}} = \begin{cases} 2.05 \text{ Å} < r_{\text{O-He}} < 10.0 \text{ Å} \\ 1.25 \text{ Å} < r_{\text{H-He}} < 10.0 \text{ Å} \end{cases} \tag{S2}$$

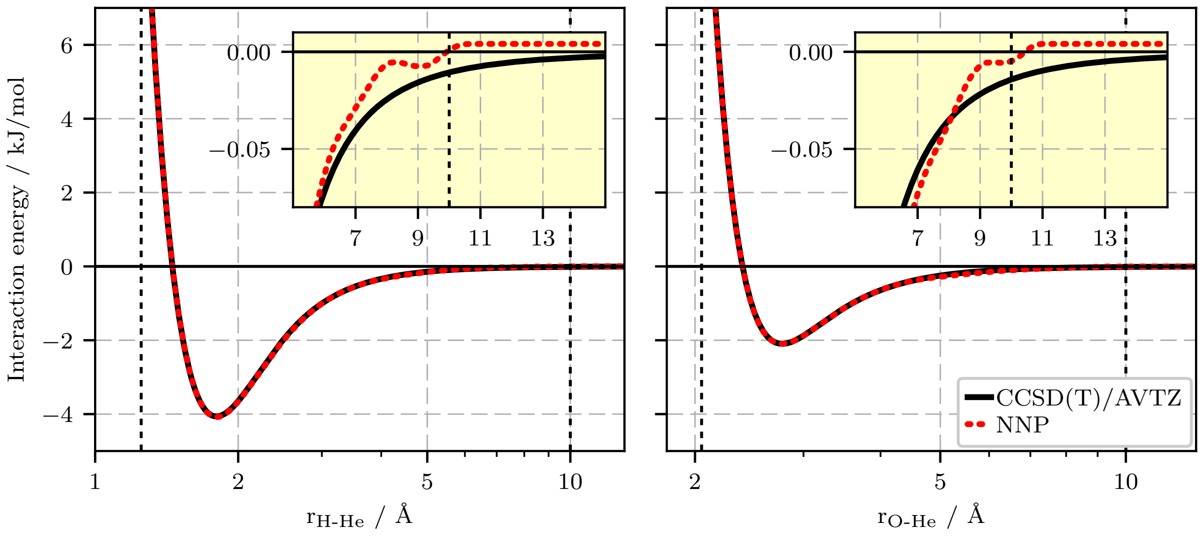


Figure S3. Interaction energy of one helim atom and the $H_3O^+$ minimum energy structure from radial scans in direction of the oxygen-hydrogen bond obtained with CCSD(T) and the AVTZcp basis as well as the predicted interaction energy from the NNP. The cutoff radii are shown as dashed black lines and the insets show a close up of the long range convergence.

that are also shown in Fig. S3. The very repulsive interactions closer than the lower cutoff are described by a Lennard-Jones term

$$E_{\text{int}}(r_{\text{X-He}}) = \left(\frac{1}{r_{\text{X-He}}}\right)^{12} \quad , \tag{S3}$$

if ever encountered during the equilibration phase of the simulation, where He atoms can be initialized too close to the solute atoms. It was ensured that no helium is closer than the lower bound cutoff in the actual production simulations. The figure also features the predicted interaction energy using the final neural network potential (NNP) along with the CCSD(T) interaction energy. This prediction agrees almost perfectly with the reference method over the whole range of distances. Only close to the long distance cutoff small deviations are present which become only visible when greatly zooming in (see insets). This could be eliminated by additionally targeting the forces during the fit of the NNP [6]. However, CCSD(T) forces are only available by numerical differentiation and impose rather high computational demands. In addition, the region that features the deviations usually lies outside the range of distances encountered in the simulations of bulk helium in truncated octahedron boundary conditions. Note that by construction, beyond the cutoff the NNP

produces a constant energy independent of the distance. This constant energy corresponds to the average energy of all training points beyond the cutoff.

### C. Box Convergence for Solvation in Bulk Helium

Simulations of quantum bulk helium, as presented in the main text, can become expensive in particular when adding bosonic exchange (which was therefore not done in this NNP study, albeit it could be added within the same code [7] to produce a superfluid quantum solvent [8]). We therefore chose a specific box size that allows us to study the solvation of solutes including the second helium solvation shell. To evaluate how many helium atoms should be simulated in the truncated octahedral supercell, we performed simulations with 256 helium atoms and set the density to the experimental value according to the phase diagram under the chosen conditions of $\rho = 0.021855$ Å$^{-3}$ at 1.67 K. These simulations serve as reference for a comparison of the RDFs with smaller numbers of helium atoms in order to determine a compromise number of helium atoms. Note that we chose to evaluate the helium-solute interaction by the nearest neighbor approach for fixed solute structures only in order to minimize the computational cost. This is justified under the assumption that structures close to the minimum energy configuration make up the largest contribution of the solute ensemble. The O-He RDFs of these convergence tests are depicted in Fig. S4 for both the $H_3O^+$ and $H_5O_2{}^+$ complex. In the case of $H_3O^+$, 98 helium atoms in the smaller box give the best agreement in the first hydration shell to the reference RDF of the larger box. However, the second hydration shell is better described by simulating 102 helium atoms in the smaller box. For the $H_5O_2{}^+$ species, simulations with 88 helium atoms match the RDF of the box with 256 helium atoms best in both hydration shells.

This conclusion is also backed up by the H-He RDFs, shown in Fig. S5, which provide a better overview over the fine structure in the first helium solvation shell. Again the first shell is described better with 98 helium atoms for hydronium, while 88 atoms give the best results for the Zundel cation. From these convergence tests we therefore conclude to use 98 helium atoms in case of the $H_3O^+$ species, while using 88 atoms for $H_5O_2{}^+$ which underlies all data shown in the main text.

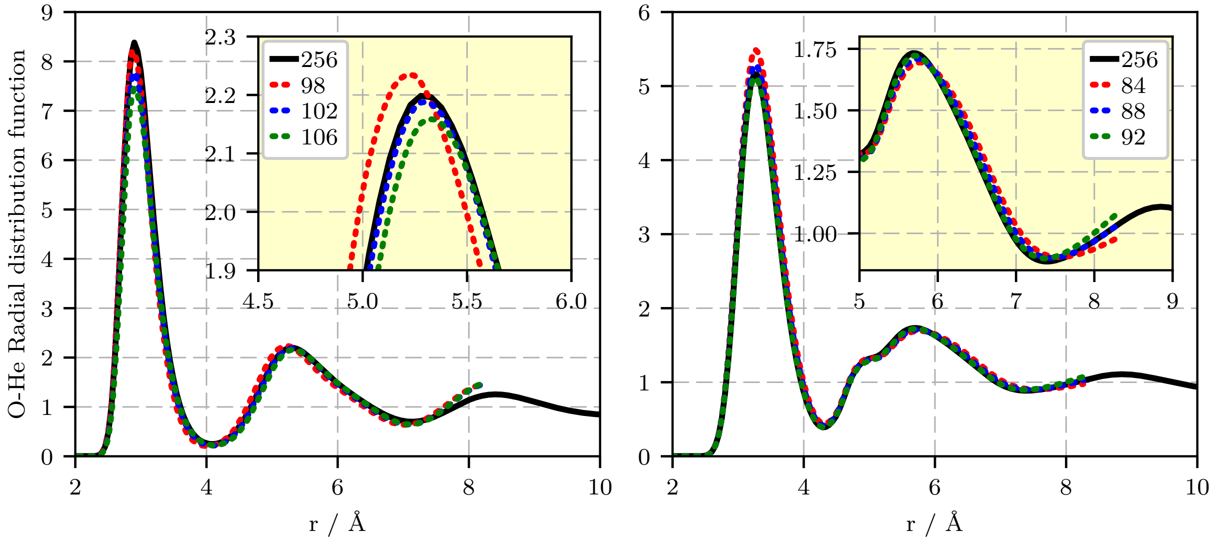


Figure S4. Oxygen-helium radial distribution functions of selected $H_3O^+$ (left) and $H_5O_2^+$ (right) structures close to their minimum energy configuration in bulk helium at 1.67 K obtained from PIMC simulations using different numbers of helium atoms around the frozen solute structures where the interaction potential was evaluated on a grid.

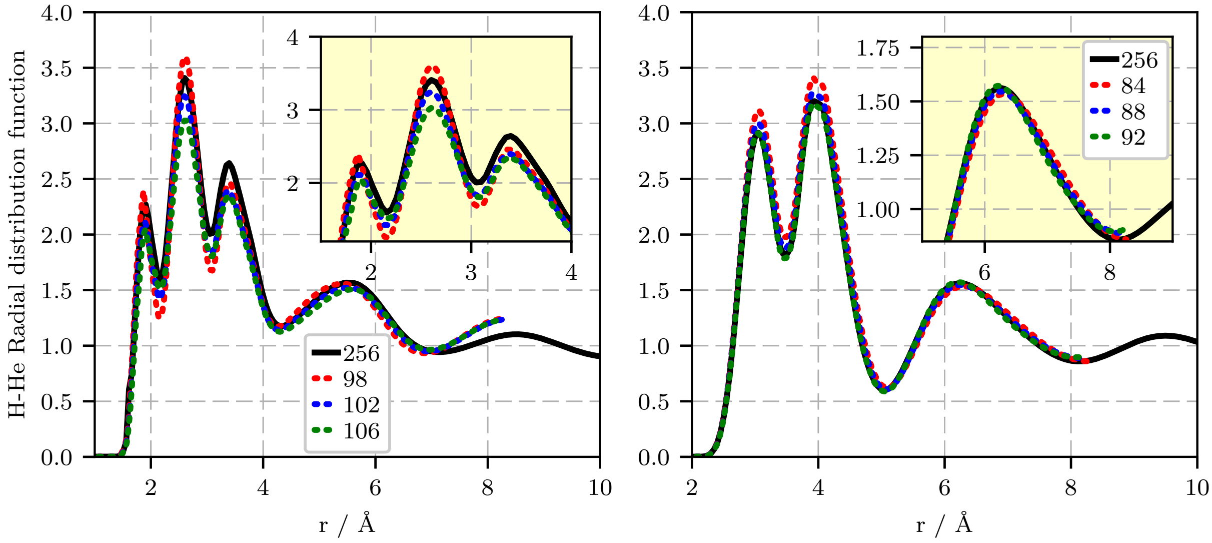


Figure S5. Hydrogen-helium radial distribution functions of selected $H_3O^+$ (left) and $H_5O_2^+$ (right) structures close to their minimum energy configuration in bulk helium at 1.67 K obtained from PIMC simulations using different numbers of helium atoms around the frozen solute structures where the interaction potential was evaluated on a grid.

### D. Symmetry Function Setup

The parameters of the radial and angular functions for He-hydronium can be found in Table I and Table III, respectively, whereas the symmetry function parameters for He-Zundel are specified in Table II and Table IV, see main text for background. Note that in contrast to other NNPs we chose different cutoffs depending on the specific atom pairs and triples to account for the varying range of distances for solute and He-solute atom pairs.

Table I. Parameters of the radial symmetry functions of type $G^2$ describing the environment of the hydrogen, helium and oxygen atoms, respectively, for each possible neighboring element in the He-hydronium NNP. A radial shift $R_{\text{shift}} = 0.0$ Bohr has been used for all symmetry functions.

| number | central atom | neighbor | $\eta$ [Bohr$^{-2}$] | $R_\text{c}$ [Bohr] |
|---|---|---|---|---|
| 1 | H | H | 0.00000 | 6.0 |
| 2 | | | 0.01284 | 6.0 |
| 3 | | | 0.04711 | 6.0 |
| 4 | | | 0.11421 | 6.0 |
| 5 | | | 0.38554 | 6.0 |
| 6 | | | 1.14214 | 6.0 |
| 7 | | He | 0.00000 | 20.0 |
| 8 | | | 0.01284 | 20.0 |
| 9 | | | 0.04711 | 20.0 |
| 10 | | | 0.11421 | 20.0 |
| 11 | | | 0.38554 | 20.0 |
| 12 | | | 1.14214 | 20.0 |
| 13 | | O | 0.00000 | 4.0 |
| 14 | | | 0.01284 | 4.0 |
| 15 | | | 0.04711 | 4.0 |
| 16 | | | 0.11421 | 4.0 |
| 17 | | | 0.38554 | 4.0 |
| 18 | | | 1.14214 | 4.0 |
| 1 | He | H | 0.00000 | 20.0 |
| 2 | | | 0.01284 | 20.0 |
| 3 | | | 0.04711 | 20.0 |
| 4 | | | 0.11421 | 20.0 |
| 5 | | | 0.38554 | 20.0 |
| 6 | | | 1.14214 | 20.0 |
| 7 | | O | 0.00000 | 20.0 |
| 8 | | | 0.01284 | 20.0 |
| 9 | | | 0.04711 | 20.0 |
| 10 | | | 0.11421 | 20.0 |
| 11 | | | 0.38554 | 20.0 |
| 1 | O | H | 0.00000 | 4.0 |
| 2 | | | 0.01284 | 4.0 |
| 3 | | | 0.04711 | 4.0 |
| 4 | | | 0.11421 | 4.0 |
| 5 | | | 0.38554 | 4.0 |
| 6 | | | 1.14214 | 4.0 |
| 7 | | He | 0.00000 | 20.0 |
| 8 | | | 0.01284 | 20.0 |
| 9 | | | 0.04711 | 20.0 |
| 10 | | | 0.11421 | 20.0 |
| 11 | | | 0.38554 | 20.0 |

Table II. Parameters of the radial symmetry functions of type $G^2$ describing the environment of the hydrogen, helium and oxygen atoms, respectively, for each possible neighboring element in the He-Zundel NNP. A radial shift $R_{\text{shift}} = 0.0$ Bohr has been used for all symmetry functions.

| number | central atom | neighbor | $\eta$ [Bohr$^{-2}$] | $R_c$ [Bohr] |
|---|---|---|---|---|
| 1 | H | H | 0.00000 | 10.0 |
| 2 | | | 0.04711 | 10.0 |
| 3 | | | 0.11421 | 10.0 |
| 4 | | | 0.38554 | 10.0 |
| 5 | | | 1.14214 | 10.0 |
| 6 | | He | 0.00000 | 20.0 |
| 7 | | | 0.04711 | 20.0 |
| 8 | | | 0.11421 | 20.0 |
| 9 | | | 0.38554 | 20.0 |
| 10 | | | 1.14214 | 20.0 |
| 11 | | O | 0.00000 | 10.0 |
| 12 | | | 0.04711 | 10.0 |
| 13 | | | 0.38554 | 10.0 |
| 14 | | | 1.14214 | 10.0 |
| 1 | He | H | 0.00000 | 20.0 |
| 2 | | | 0.04711 | 20.0 |
| 3 | | | 0.11421 | 20.0 |
| 4 | | | 0.38554 | 20.0 |
| 5 | | | 1.14214 | 20.0 |
| 6 | | O | 0.00000 | 20.0 |
| 7 | | | 0.04711 | 20.0 |
| 8 | | | 0.11421 | 20.0 |
| 9 | | | 0.38554 | 20.0 |
| 1 | O | H | 0.00000 | 10.0 |
| 2 | | | 0.04711 | 10.0 |
| 3 | | | 0.11421 | 10.0 |
| 4 | | | 0.38554 | 10.0 |
| 5 | | | 1.14214 | 10.0 |
| 6 | | He | 0.00000 | 20.0 |
| 7 | | | 0.04711 | 20.0 |
| 8 | | | 0.11421 | 20.0 |
| 9 | | | 0.38554 | 20.0 |
| 10 | | O | 0.00000 | 8.0 |

Table III. Parameters of the angular symmetry functions of type $G^4$ describing the environment of each atom with respect to the elements of the neighboring atom in the He-hydronium NNP. A value of $\eta = 0.0$ Bohr$^{-2}$ has been used for all symmetry functions.

| number | central atom | neighbor | $\lambda$ | $\zeta$ | $R_c$ [Bohr] |
|---|---|---|---|---|---|
| 19 | H | H He | 1.0 | 2.0 | 20.0 |
| 20 | | | 1.0 | 16.0 | 20.0 |
| 21 | | | -1.0 | 2.0 | 20.0 |
| 22 | | | -1.0 | 16.0 | 20.0 |
| 23 | | H O | 1.0 | 2.0 | 6.0 |
| 24 | | | 1.0 | 16.0 | 6.0 |
| 25 | | | -1.0 | 2.0 | 6.0 |
| 12 | He | H H | 1.0 | 2.0 | 20.0 |
| 13 | | | 1.0 | 16.0 | 20.0 |
| 14 | | | -1.0 | 2.0 | 20.0 |
| 15 | | H O | 1.0 | 2.0 | 20.0 |
| 16 | | | 1.0 | 16.0 | 20.0 |
| 17 | | | -1.0 | 2.0 | 20.0 |
| 12 | O | H H | 1.0 | 2.0 | 6.0 |
| 13 | | | -1.0 | 2.0 | 6.0 |
| 14 | | | -1.0 | 16.0 | 6.0 |
| 15 | | H He | 1.0 | 2.0 | 20.0 |
| 16 | | | 1.0 | 16.0 | 20.0 |
| 17 | | | -1.0 | 2.0 | 20.0 |
| 18 | | | -1.0 | 16.0 | 20.0 |

Table IV. Parameters of the angular symmetry functions of type $G^4$ describing the environment of each atom with respect to the elements of the neighboring atom in the He-Zundel NNP. A value of $\eta = 0.0$ Bohr$^{-2}$ has been used for all symmetry functions.

| number | central atom | neighbor | $\lambda$ | $\zeta$ | $R_c$ [Bohr] |
|---|---|---|---|---|---|
| 15 | H | H He | 1.0 | 2.0 | 20.0 |
| 16 | | | 1.0 | 8.0 | 20.0 |
| 17 | | | 1.0 | 16.0 | 20.0 |
| 18 | | | -1.0 | 2.0 | 20.0 |
| 19 | | | -1.0 | 8.0 | 20.0 |
| 20 | | | -1.0 | 16.0 | 20.0 |
| 21 | | He O | 1.0 | 2.0 | 20.0 |
| 22 | | | 1.0 | 8.0 | 20.0 |
| 23 | | | 1.0 | 16.0 | 20.0 |
| 24 | | | -1.0 | 2.0 | 20.0 |
| 25 | | | -1.0 | 8.0 | 20.0 |
| 26 | | | -1.0 | 16.0 | 20.0 |
| 27 | | H O | 1.0 | 2.0 | 10.0 |
| 28 | | | 1.0 | 16.0 | 10.0 |
| 29 | | | -1.0 | 2.0 | 10.0 |
| 30 | | | -1.0 | 16.0 | 10.0 |
| 31 | | O O | 1.0 | 2.0 | 10.0 |
| 32 | | | 1.0 | 16.0 | 10.0 |
| 33 | | | -1.0 | 2.0 | 10.0 |
| 34 | | | -1.0 | 16.0 | 10.0 |
| 10 | He | H H | 1.0 | 2.0 | 20.0 |
| 11 | | | 1.0 | 16.0 | 20.0 |
| 12 | | | -1.0 | 2.0 | 20.0 |
| 13 | | | -1.0 | 16.0 | 20.0 |
| 14 | | H O | 1.0 | 2.0 | 20.0 |
| 15 | | | 1.0 | 16.0 | 20.0 |
| 16 | | | -1.0 | 2.0 | 20.0 |
| 17 | | | -1.0 | 16.0 | 20.0 |
| 18 | | O O | 1.0 | 2.0 | 20.0 |
| 19 | | | -1.0 | 2.0 | 20.0 |
| 11 | O | H H | 1.0 | 2.0 | 10.0 |
| 12 | | | 1.0 | 16.0 | 10.0 |
| 13 | | | -1.0 | 2.0 | 10.0 |
| 14 | | | -1.0 | 16.0 | 10.0 |
| 15 | | H O | 1.0 | 2.0 | 10.0 |
| 16 | | | 1.0 | 16.0 | 10.0 |
| 17 | | | -1.0 | 2.0 | 10.0 |
| 18 | | | -1.0 | 16.0 | 10.0 |
| 19 | | H He | 1.0 | 2.0 | 10.0 |
| 20 | | | 1.0 | 8.0 | 20.0 |
| 21 | | | 1.0 | 16.0 | 20.0 |
| 22 | | | -1.0 | 2.0 | 20.0 |
| 23 | | | -1.0 | 8.0 | 20.0 |
| 24 | | | -1.0 | 16.0 | 20.0 |
| 25 | | He O | 1.0 | 2.0 | 20.0 |
| 26 | | | -1.0 | 2.0 | 20.0 |

## II. SUPPLEMENTAL ANALYSES AND RESULTS

In the following the additional spatial distribution functions (SDFs) of helium around selected, clamped solute structures are presented as comparison between the reference method and the neural network interaction potential. Since we are not aiming at understanding the solvation structure in the present work, but performed the calculations as a test for our NNP methodology, the comparison is given without further explanations and should simply highlight the substantial agreement between the CCSD(T)/AVTZcp reference data and the interaction energies as obtained from the fully trained NNPs as a tiny fraction of computational cost. Cases where minor deviations are present are discussed in detail in the main text.

## A. Helium Microsolvation

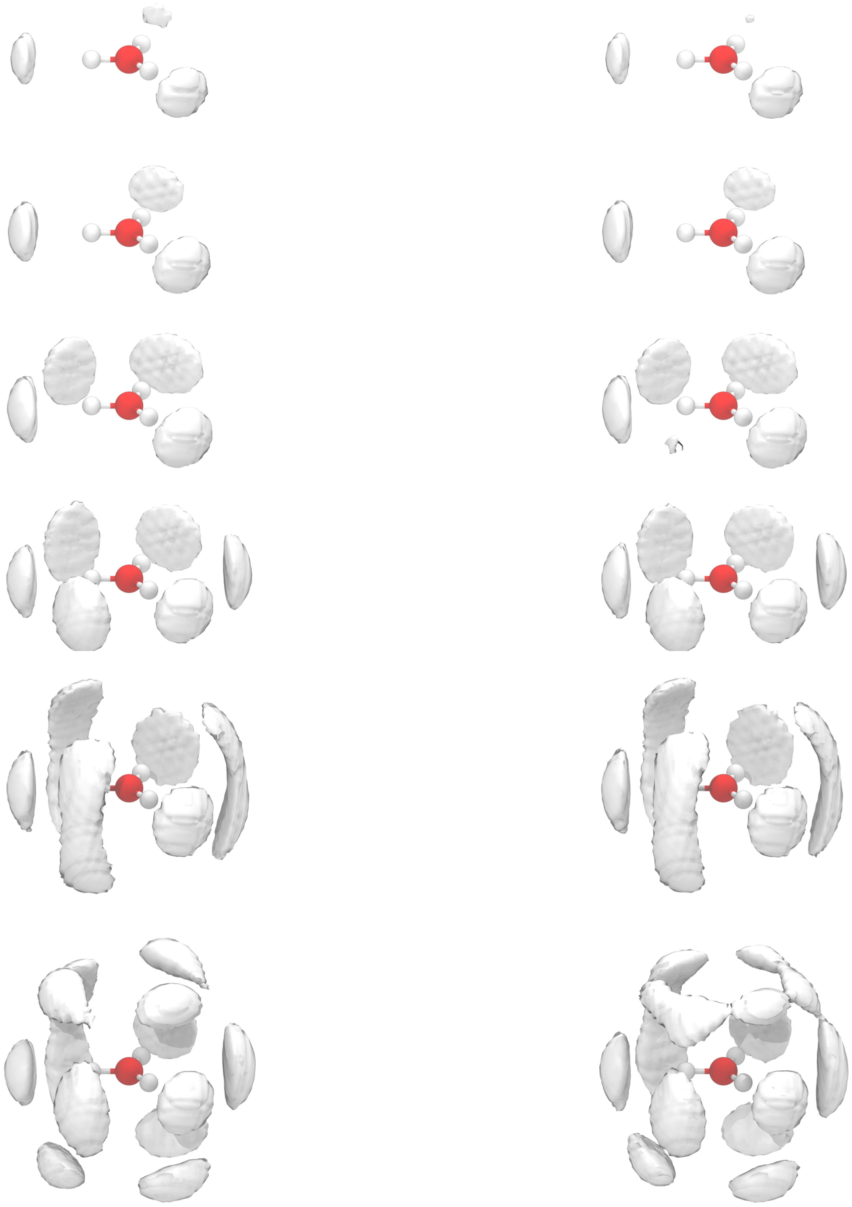

Figure S6. Comparison of helium SDFs obtained from path integral simulations with (from top to bottom) 1, 2, 4, 6, 10 and 14 helium atoms in the field of a static $H_3O^+$ molecule in a flat orientation. Left: Energies obtained from the coupled cluster grid. Right: NNP evaluated at the coupled cluster grid points. The isovalue is the same in all shown cases.

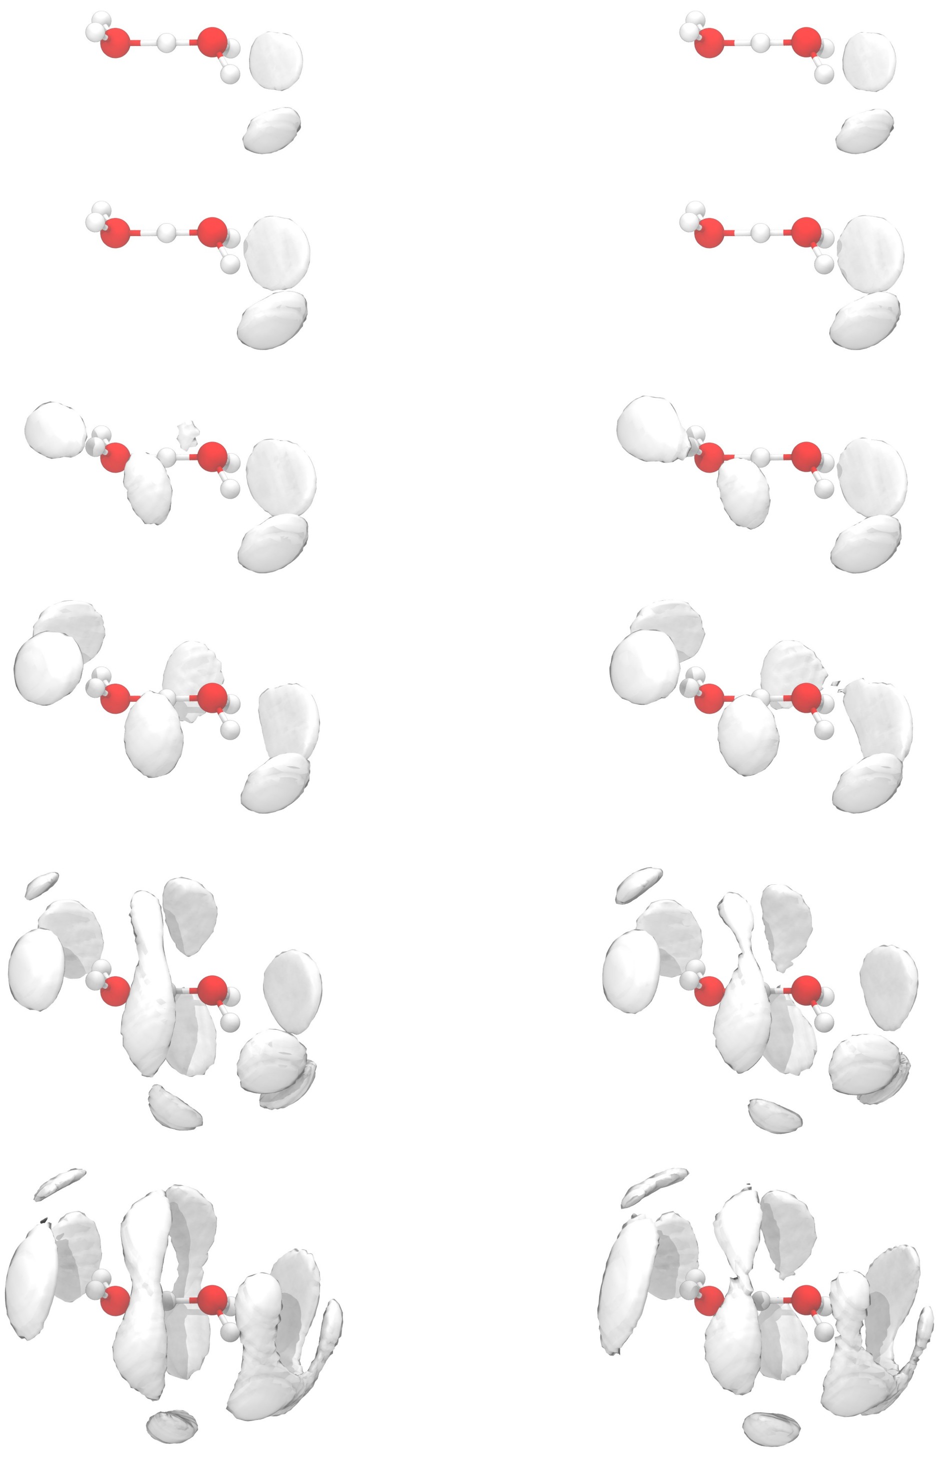

Figure S7. Comparison of helium SDFs obtained from path integral simulations with (from top to bottom) 1, 2, 4, 6, 10 and 14 helium atoms in the field of a static ${H_5O_2}^+$ molecule close to its minimum energy configuration. Left: Energies obtained from the coupled cluster grid. Right: NNP evaluated at the coupled cluster grid points. The isovalue is the same in all shown cases.

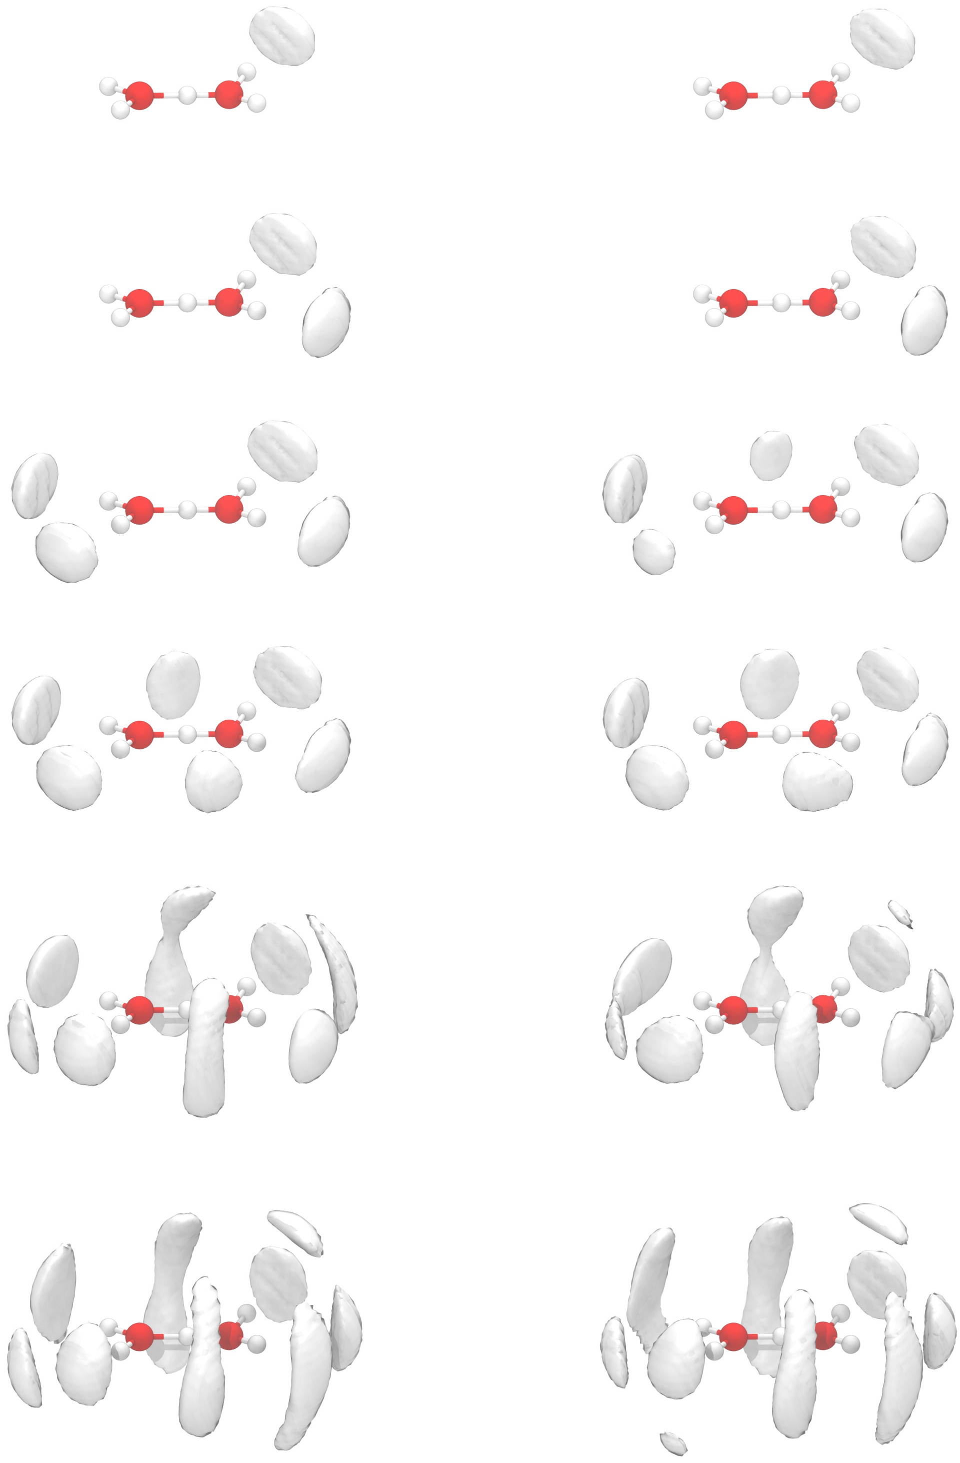

Figure S8. Comparison of helium SDFs obtained from path integral simulations with (from top to bottom) 1, 2, 4, 6, 10 and 14 helium atoms in the field of a static $H_5O_2{}^+$ molecule in a flat orientation. Left: Energies obtained from the coupled cluster grid. Right: NNP evaluated at the coupled cluster grid points. The isovalue is the same in all shown cases.

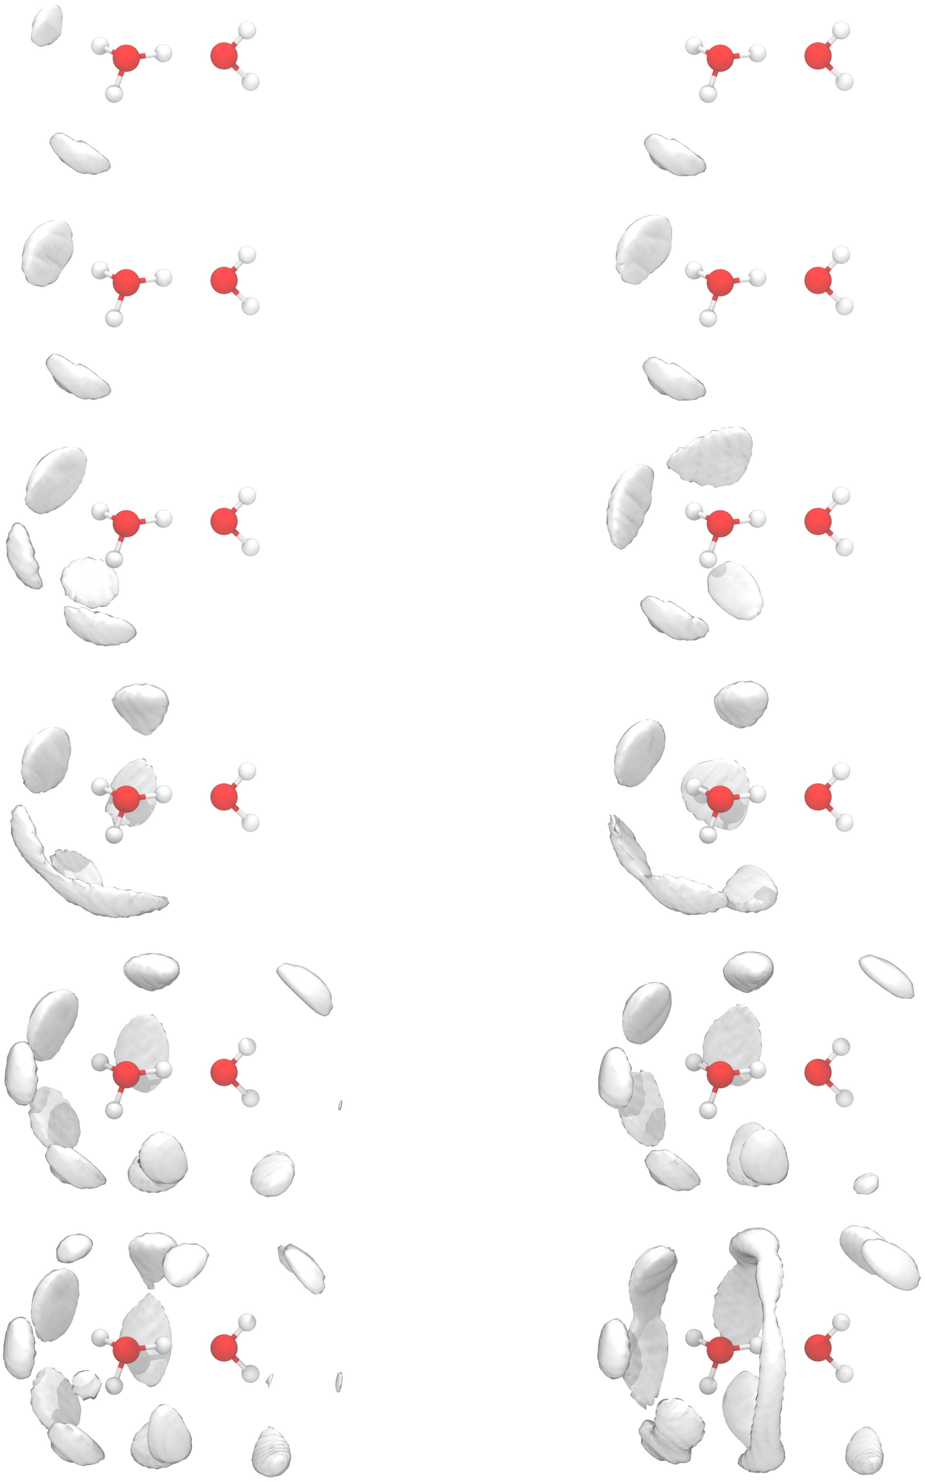

Figure S9. Comparison of helium SDFs obtained from path integral simulations with (from top to bottom) 1, 2, 4, 6, 10 and 14 helium atoms in the field of a static $H_5O_2^+$ molecule in an asymmetric proton transfer situation. Left: Energies obtained from the coupled cluster grid. Right: NNP evaluated at the coupled cluster grid points. The isovalue is the same in all shown cases.

## B. Helium Bulk Solvation

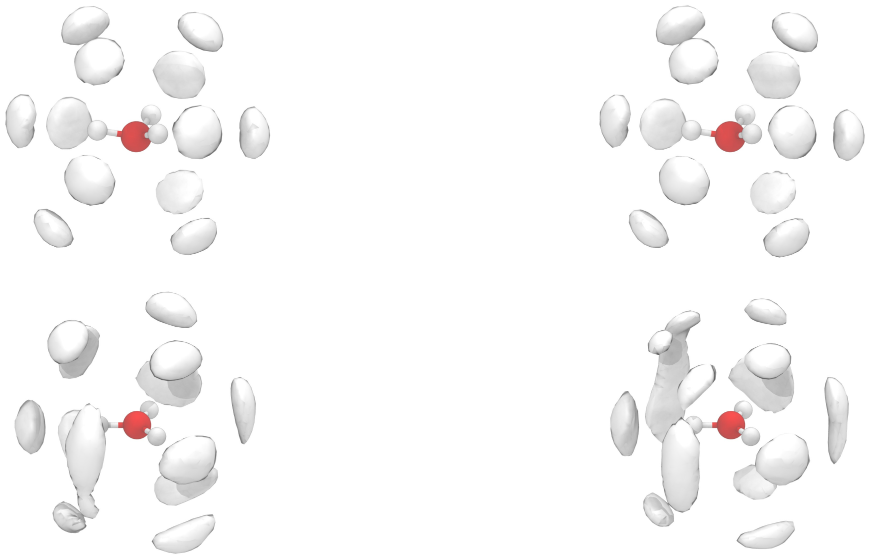

Figure S10. Comparison of helium SDFs obtained from path integral simulations with 98 helium atoms in the field of a static $H_3O^+$ molecule close to its minimum energy geometry (top) and in a flat configuration (bottom) centered in a truncated octahedron cell. Left: Energies obtained from the coupled cluster grid. Right: NNP evaluated at the coupled cluster grid points. The isovalue is the same in all shown cases.

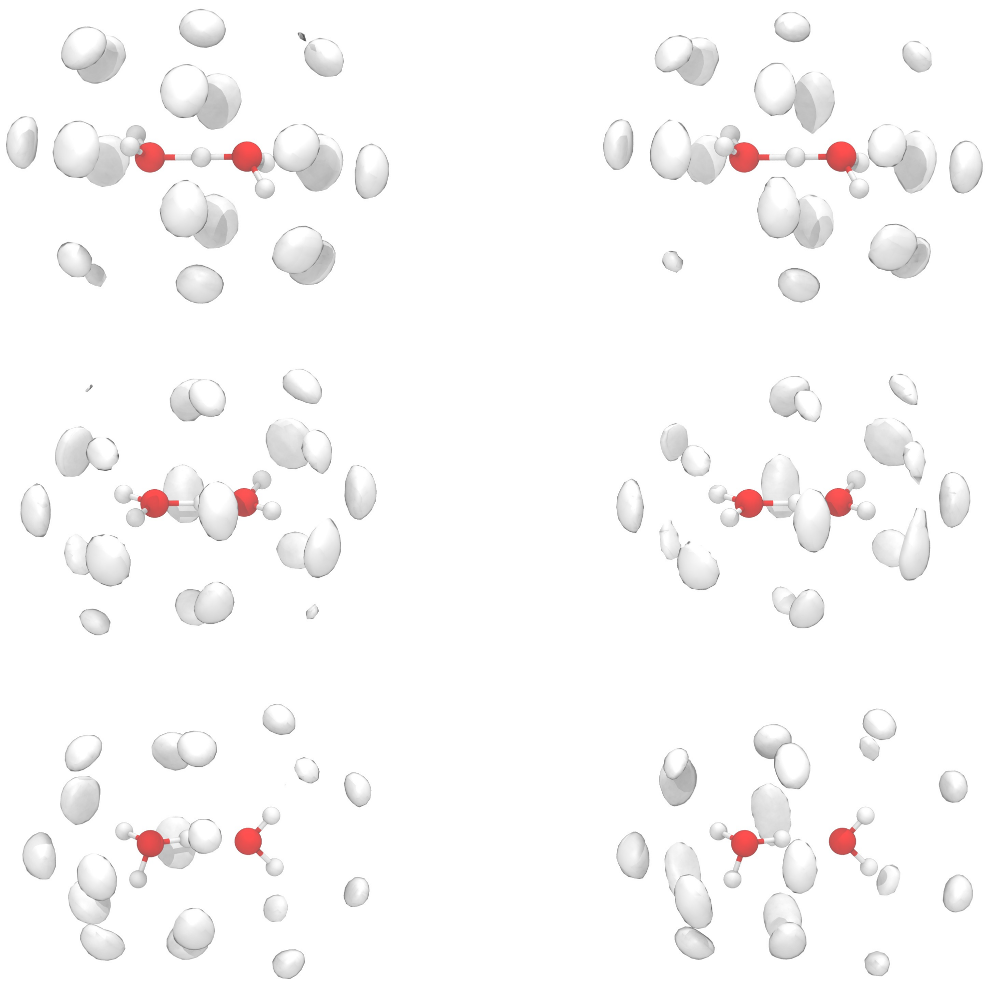

Figure S11. Comparison of helium SDFs obtained from path integral simulations with 88 helium atoms in the field of a static ${H_5O_2}^+$ molecule in a selected configuration close to the minimum energy geometry (top), in a flat orientation (middle) as well as in an asymmetric proton transfer situation (bottom) centered in a truncated octahedron cell. Left: Energies obtained from the coupled cluster grid. Right: NNP evaluated at the coupled cluster grid points. The isovalue is the same in all shown cases.

## C. Estimation of Statistical Accuracy

In order to estimate the statistical accuracy of the SDFs shown in the previous sections herein as well as in the manuscript, we conducted two additional simulations with ten times enhanced statistics for the case of 14 helium atoms around the flat hydronium configuration both for the NNP and CCSD(T) grid. Note that this results in averaging over $10^9$ configurations for each SDF. The comparison of the resulting SDFs with the previously generated ones is depicted in Fig. S12. The SDFs are essentially equivalent for both simulation lengths and we therefore conclude that the properties presented in the main text and in earlier sections are statistically converged.

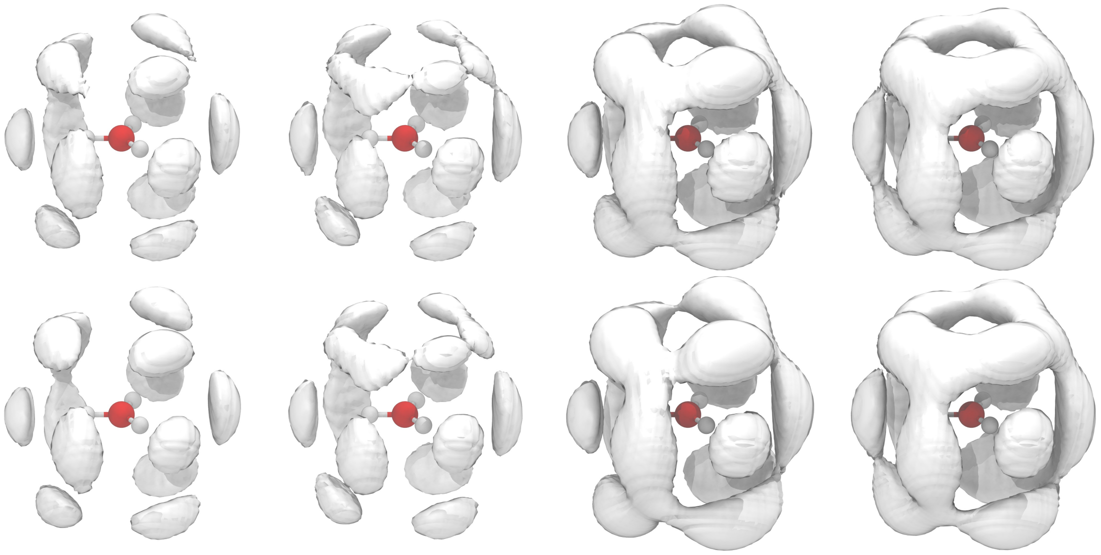

Figure S12. Comparison of helium SDFs with different simulation length obtained from path integral simulations with 14 helium atoms in the field of a frozen $H_3O^+$ configuration in a flat orientation ('Flat'). First and third column: Energies obtained from the coupled cluster grid. Second and fourth column: NNP evaluated at the coupled cluster grid points. First and second column: isovalue = $0.2{\cdot}10^{-3}$ 1/bohr$^3$. Third and fourth column: isovalue = $0.08{\cdot}10^{-3}$ 1/bohr$^3$; note that the SDFs have been normalized to the number of helium atoms. First row: Simulation length as described in the main text. Second row: Ten times improved simulation length.

[1] C. Schwartz, *Phys. Rev.* **1962**, *126*, 1015–1019.

[2] R. A. Kendall, T. H. J. Dunning, R. J. Harrison, *J. Chem. Phys.* **1992**, *96*, 6796–6806.

[3] D. E. Woon, T. H. Dunning Jr., *J. Chem. Phys.* **1994**, *100*, 2975–2988.

[4] S. F. Boys, F. Bernardi, *Mol. Phys.* **1970**, *19*, 553–566.

[5] X. Sheng, F. Hu, S. Qian, *Comput. Theor. Chem.* **2017**, *1102*, 1–4.

[6] J. Behler, *J. Chem. Phys.* **2011**, *134*, 074106.

[7] L. Walewski, H. Forbert, D. Marx, *Comput. Phys. Commun.* **2014**, *185*, 884–899.

[8] L. Walewski, H. Forbert, D. Marx, *J. Chem. Phys.* **2014**, *140*, 144305.
